# Supplementary material for: Machine Learning Photodynamics Unveils a Controlled H$_2$ Loss Channel in Methaniminium Cation
Source: arXiv:2512.00913 source file (2025-11-30)
Supplement: Supplementary file 1 [file SI.pdf]

# Supporting Information: Machine Learning Photodynamics Unveils a Controlled $H_2$ Loss Channel in Methaniminium Cation

Daniil N. Chistikov,[†,¶] Pavel M. Radzikovitsky,[†] Dmitry S. Popov,[†] Ivan V. Dudakov,[†,‡] Vadim V. Korolev,[†,‡] Vladimir E. Bochenkov,[†] and Anastasia V. Bochenkova[*,†]

†*Department of Chemistry, Lomonosov Moscow State University, Leninskie Gory 1/3, 119991 Moscow, Russia*

‡*MSU Institute for Artificial Intelligence, Lomonosov Moscow State University, Moscow 119192, Russia*

¶*Institute of Quantum Physics, Irkutsk National Research Technical University, 83 Lermontov Street, Irkutsk 664074, Russia*

E-mail: bochenkova@phys.chem.msu.ru

# Contents


**1 Vertical transitions** **S-3**

**2 Geometries of the conical intersections** **S-4**

**3 CASSCF topography around MECIs** **S-5**

**4 CASSCF and XMCQDPT2 energy scans** **S-6**

**5 Franck-Condon active vibrational modes** **S-9**

**6 Nonadiabatic dynamics simulations** **S-10**

**7 Dataset construction and neural network potentials** **S-12**

**8 Analysis of photodissociation channels** **S-14**

**9 Temporal evolution of photodissociation channels** **S-19**

**10 ML analysis of excited-state decay through MECIs** **S-20**

10.1 Locating MECIs with the ML potential . . . . . . . . . . . . . . . . . . . . . . S-20

10.2 Geometries of MECIs from the ML potential . . . . . . . . . . . . . . . . . . . S-21

10.3 Energies of MECIs from the ML potential . . . . . . . . . . . . . . . . . . . . S-22

10.4 Statistical uncertainty of the ML-based branching ratios . . . . . . . . . . . S-22

**11 Ab initio and ML population dynamics** **S-23**

**12 Assessing robustness in ML dynamics** **S-24**

**13 Branching ratios of final products from $S_1$ decay** **S-27**

**14 Infrared absorption spectrum** **S-28**

**References** **S-29**

# 1 Vertical transitions

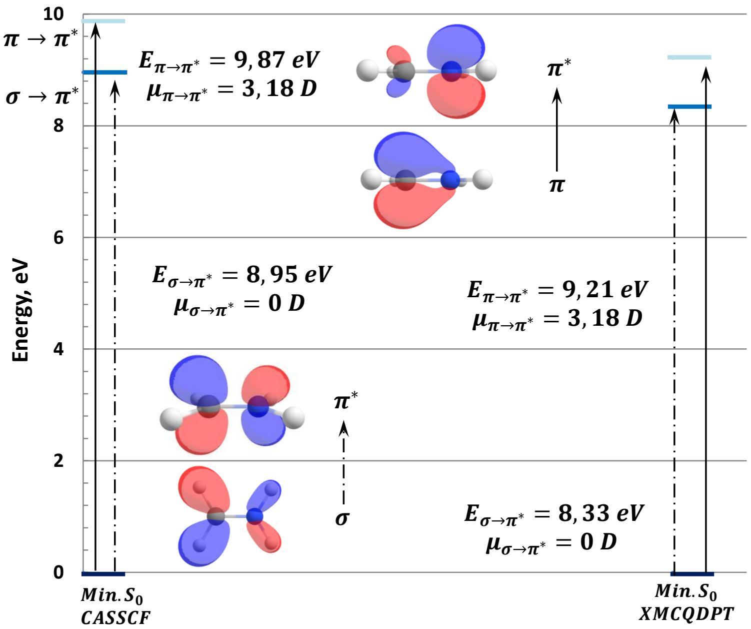


Figure S1: Vertical excitation energies and electronic transition dipole moments in the Franck-Condon region calculated at the SA(3)-CASSCF(12,12)/cc-pVDZ (left) and XMCQDPT2/SA(3)-CASSCF(12,12)/cc-pVDZ (right) levels of theory. Shown are also the natural XMCQDPT2 orbitals involved in the lowest-lying transitions. In $CH_2NH_2^+$, the lowest-energy $\sigma\pi^*$ and $\pi\pi^*$ states are both of a valence type, consistent with prior work establishing that Rydberg states lie higher in energy.[S1] The equilibrium geometry of the molecule possesses $C_{2v}$ symmetry. The $\pi\pi^*$ state ($S_2$) is of $A_1$ symmetry ($2^1A_1$), making the $S_0 \rightarrow S_2$ transition electronically allowed. In contrast, the $\sigma\pi^*$ state ($S_1$) is of $A_2$ symmetry ($1^1A_2$), rendering the $S_0 \rightarrow S_1$ transition symmetry-forbidden. Population of the $S_1$ state is nevertheless possible via a vibronically allowed transition, which is enabled by exciting vibrational modes of $A_2$, $B_1$, or $B_2$ symmetry (see Table S3 in Section 14).

## 2 Geometries of the conical intersections

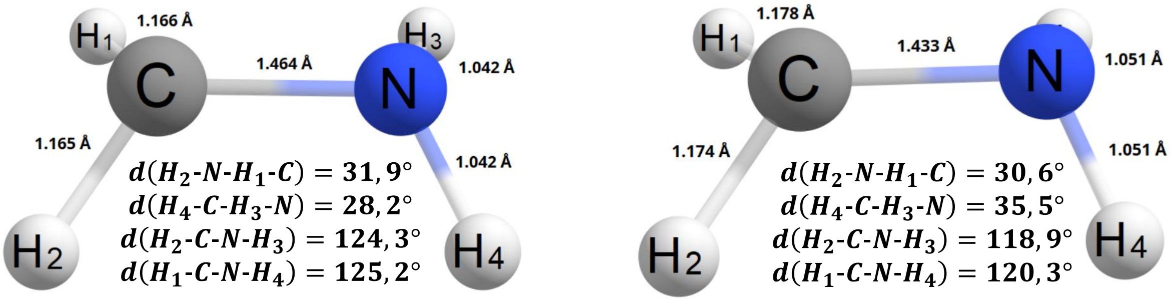


Figure S2: Geometry of the $S_2/S_1$ MECI, located using the SA(3)-CASSCF(12,12)/cc-pVDZ (left) and XMCQDPT2/SA(3)-CASSCF(12,12)/cc-pVDZ (right) methods. The root-mean-square deviation between the two structures is 0.048 Å.

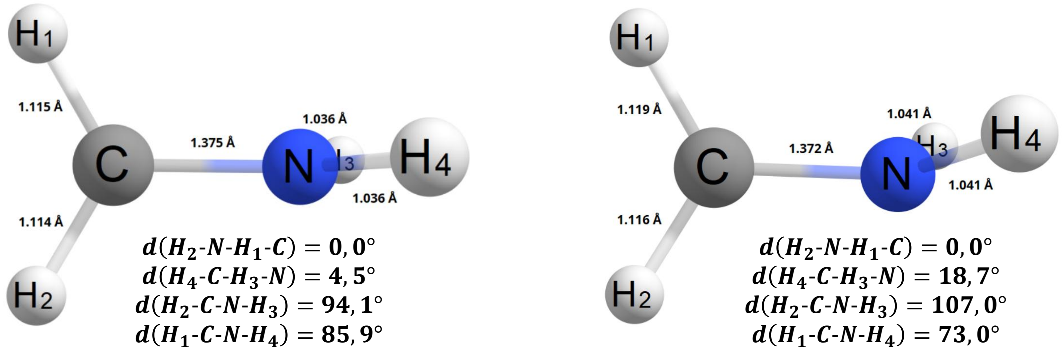


Figure S3: Geometry of the $\pi\pi^*/S_0$ MECI, located using the SA(3)-CASSCF(12,12)/cc-pVDZ (left) and XMCQDPT2/SA(3)-CASSCF(12,12)/cc-pVDZ (right) methods. The root-mean-square deviation between the two structures is 0.064 Å.

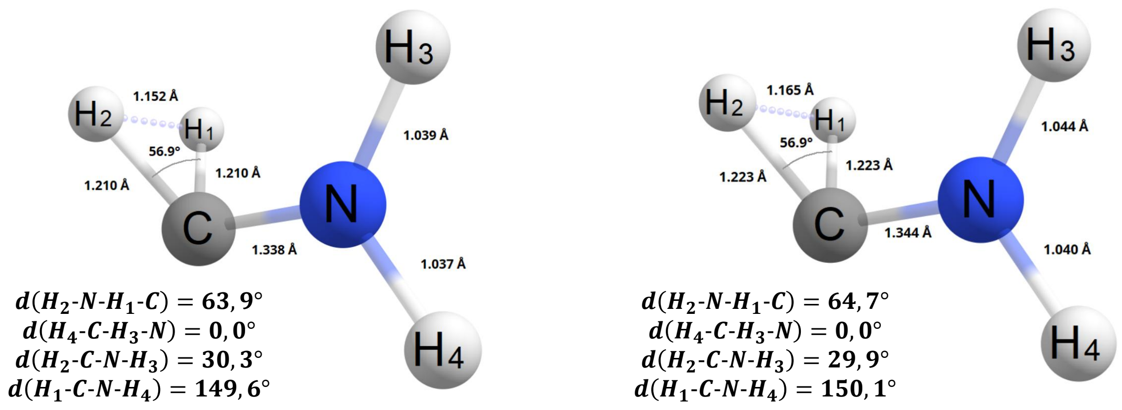


Figure S4: Geometry of the $\sigma\pi^*/S_0$ MECI, located using the SA(3)-CASSCF(12,12)/cc-pVDZ (left) and XMCQDPT2/SA(3)-CASSCF(12,12)/cc-pVDZ (right) methods. The root-mean-square deviation between the two structures is 0.013 Å.

# 3 CASSCF topography around MECIs

Figure S5 shows the topographies of the potential energy surfaces around three minimum-energy conical intersections obtained using the SA(3)-CASSCF(12,12)/cc-pVDZ method. These topographies are very much alike to those obtained using the XMCQDPT2/SA(3)-CASSCF(12,12)/cc-pVDZ method. For comparison, see Fig. 2 in the main text. Note that the topographies around the $\sigma\pi^*/S_0$ and $\pi\pi^*/S_0$ are of the same peaked type.

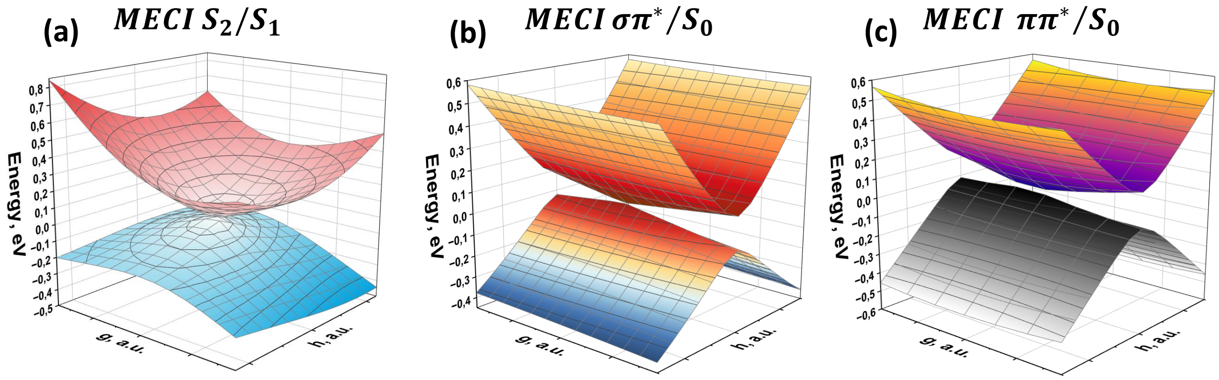


Figure S5: CASSCF topographies of the potential energy surfaces around the minimum-energy conical intersections: (a) $S_2(\pi\pi^*)/S_1(\sigma\pi^*)$ ; (b) $S_1(\sigma\pi^*)/S_0$; (c) $S_1(\pi\pi^*)/S_0$. The surfaces are plotted in the corresponding branching planes spanned by the gradient difference (g) and nonadiabatic coupling (h) vectors.

# 4 CASSCF and XMCQDPT2 energy scans

Potential energy surface scans obtained through geodesic interpolations[S2] between the Franck-Condon point and minimum-energy conical intersections using the XMCQDPT2/SA(3)-CASSCF(12,12)/cc-pVDZ level of theory are shown in Fig. S6 (from $S_1$) and Fig. S7 (from $S_2$). For comparison, Fig. S8 shows the scans starting from $S_2$ obtained with the SA(3)-CASSCF(12,12)/cc-pVDZ method. The topographies of the potential energy surfaces along the reaction coordinates obtained via the CASSCF and XMCDQPT2 methods are qualitatively similar. In particular, there are no barriers along the reaction pathways, which lead from the Franck-Condon point to the first $S_2/S_1$ MECI and further to the $\sigma\pi^*/S_0$ and $\pi\pi^*/S_0$ conical intersections. The topography of the potential energy surface along the branch, leading to the novel $\sigma\pi^*/S_0$ MECI, is very shallow after crossing the $S_2/S_1$ conical intersection. This pathway is therefore greatly disfavored when excitation starts in $S_2$, compared to the other branch, which is characterized by a steep topography towards the $\pi\pi^*/S_0$ MECI.

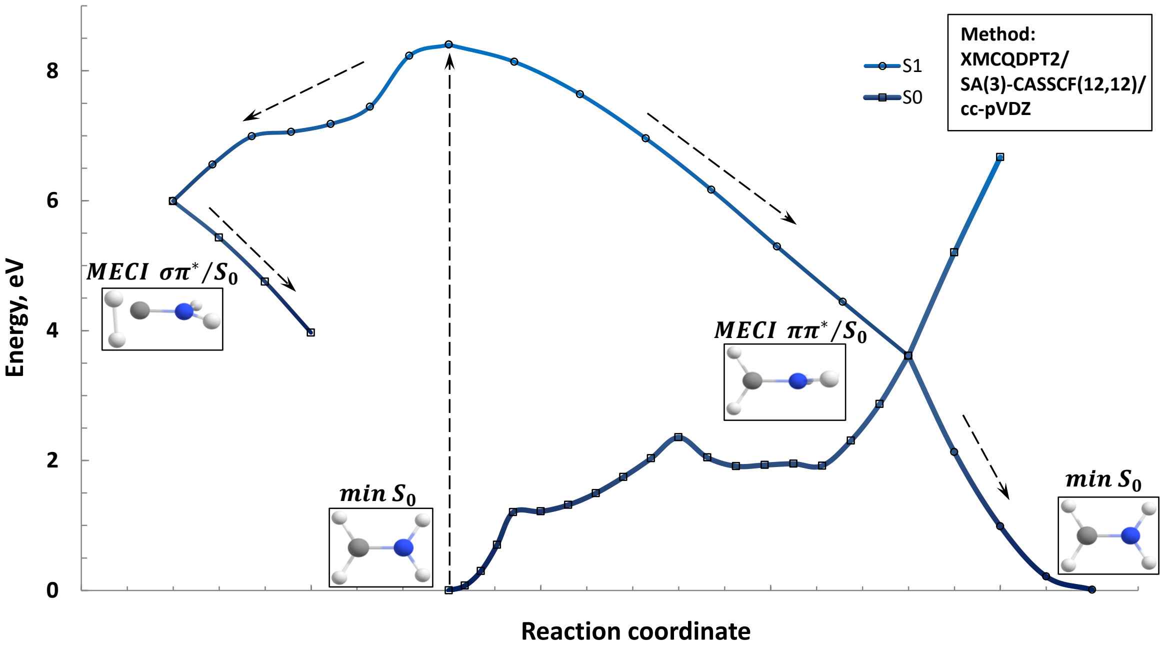


Figure S6: XMCQDPT2 potential energy surface scans obtained through geodesic interpolations[S2] between the Franck-Condon point in $S_1$ and MECI structures.

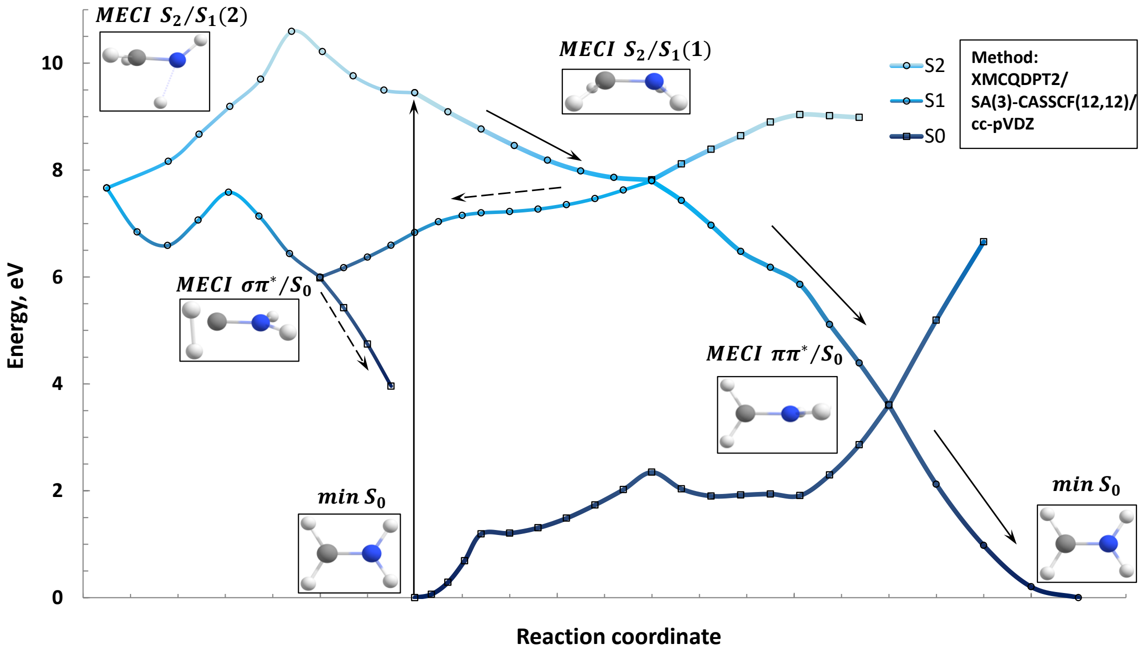


Figure S7: XMCQDPT2 potential energy surface scans obtained through geodesic interpolations[S2] between the Franck-Condon point in $S_2$ and MECI structures.

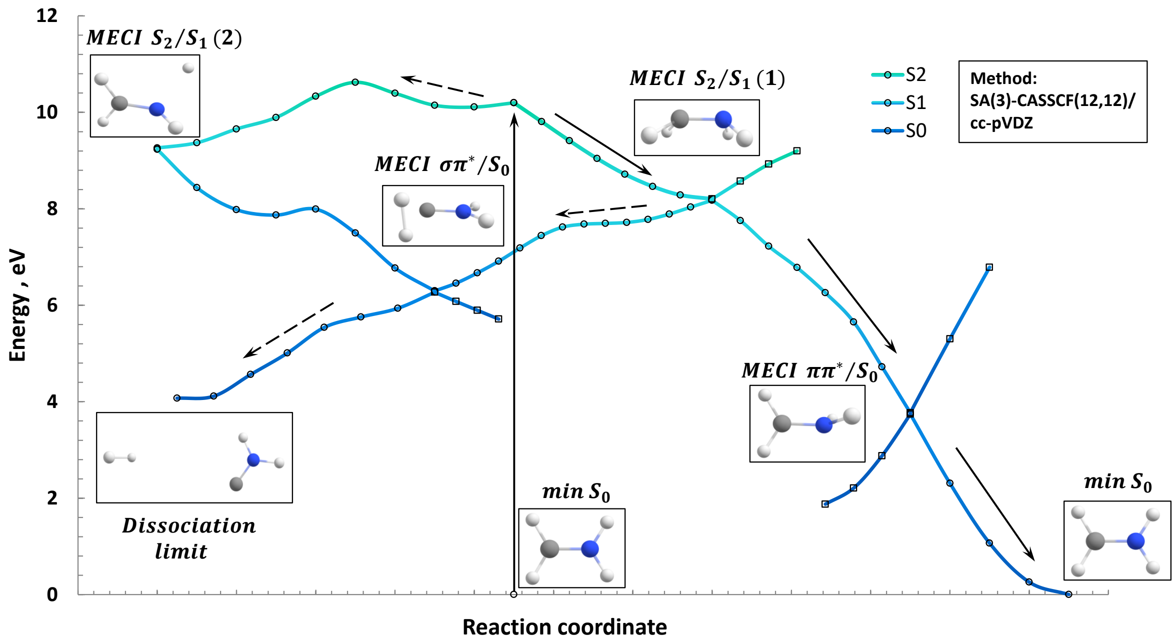


Figure S8: CASSCF potential energy surface scans obtained through geodesic interpolations[S2] between the Franck-Condon point in $S_2$ and MECI structures.

Table S1 compares the relative energies of the MECIs located with SA(3)-CASSCF(12,12)/cc-pVDZ and XMCQDPT2/SA(3)-CASSCF(12,12)/cc-pVDZ levels of theory. As expected, the lack of dynamic correlation in CASSCF yields higher relative energies. Consequently, the calculated excess energy in $CH_2NH_2^+$ is larger, leading to shorter excited-state lifetimes. However, the relative branching ratio for the $\sigma\pi^*/S_0$ and $\pi\pi^*/S_0$ pathways is expected to be similar, as the lack of dynamic correlation shifts the energies of both MECIs to a comparable degree.

Table S1: Comparison of the MECI relative energies (in eV) calculated at the SA(3)-CASSCF(12,12)/cc-pVDZ and XMCQDPT2/SA(3)-CASSCF(12,12)/cc-pVDZ levels of theory. Energies are given relative to the ground-state equilibrium geometry. Excess energies in the $CH_2NH_2^+$ molecule at the MECIs are shown with respect to the $S_0 \rightarrow S_2$ vertical excitation energy (VEE).

| | $S_2/S_1$ | $\sigma\pi^*/S_0$ | $\pi\pi^*/S_0$ |
|---|---|---|---|
| | Relative to the ground-state equilibrium geometry | | |
| CASSCF | 8.2 | 6.3 | 3.8 |
| XMCQDPT2 | 7.8 | 6.0 | 3.6 |
| | Excess energy with respect to the $S_0 \rightarrow S_2$ VEE | | |
| CASSCF | 1.7 | 3.6 | 6.1 |
| XMCQDPT2 | 1.4 | 3.2 | 5.6 |

## 5 Franck-Condon active vibrational modes

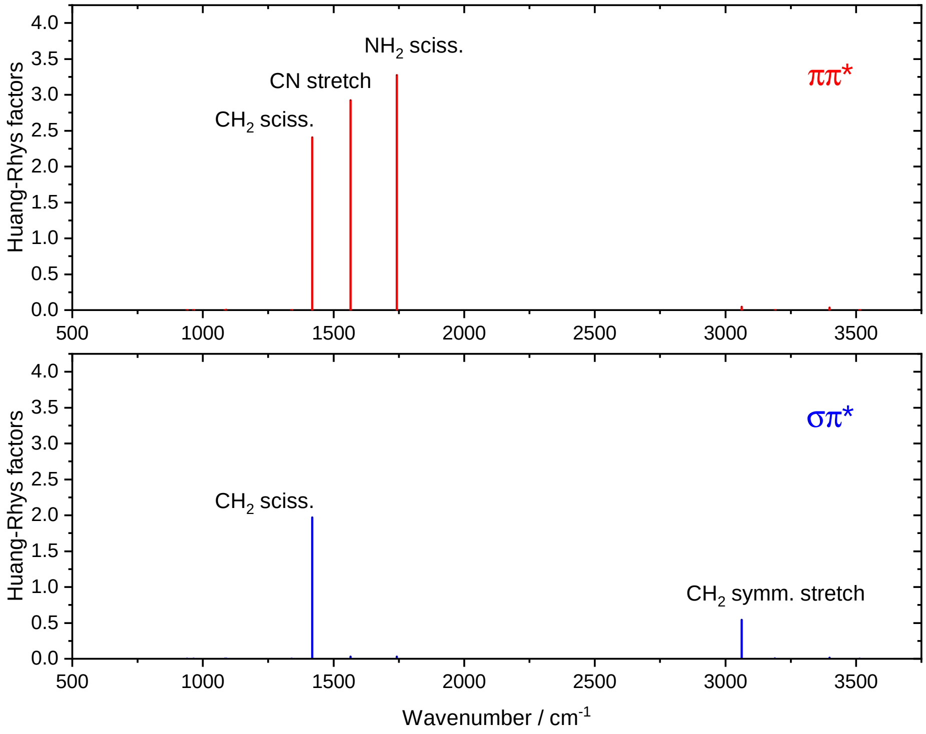


Figure S9: Franck-Condon active vibrational modes upon the $S_0 \rightarrow S_2/\pi\pi^*$ (upper panel) and $S_0 \rightarrow S_1/\sigma\pi^*$ (lower panel) transitions. Shown are the dimensionless Huang-Rhys factors calculated within the linear coupling model. Frequencies, normal modes, and vertical gradients are calculated at the SA(3)-CASSCF(12,12)/aug-cc-pVDZ level of theory.

# 6 Nonadiabatic dynamics simulations

In order to simulate the time evolution of the photoexcited methaniminium cation $CH_2NH_2^+$, we employed two commonly used approaches for simulating semiclassical nonadiabatic dynamics: Tully's fewest switches surface hopping (FSSH)[S3] and Landau-Zener surface hopping in a form proposed by Belyaev and Lebedev (LZBL).[S4]

The FSSH approach is based on the combined solution of the time-dependent Schrödinger equation for the electronic subsystem of a molecule and Newton's equations of motion for the nuclear subsystem. Representing the electronic time-dependent wave function as a linear combination of the appropriate electronic basis functions $\varphi_i$, we find for the time-evolution of the expansion coefficients $c_j(t)$:

$$i\hbar \frac{\mathrm{d}c_j(t)}{\mathrm{d}t} = \sum_i c_i(t)[H_{ji} - i\hbar \mathbf{v} \cdot \mathbf{F}_{ji}], \tag{1}$$

where $\mathbf{v}$ is the nuclear velocities vector, $H_{ji}$ and $\mathbf{F}_{ji}$ are, respectively, the matrix elements of the electronic Hamiltonian and non-adiabatic couplings (NACs):

$$H_{ji} = \langle \varphi_j | H_e | \varphi_i \rangle \,, \tag{2}$$

$$F_{ji} = \langle \varphi_j | \nabla_{\mathbf{R}} | \varphi_i \rangle \,. \tag{3}$$

The product of the velocities vector and NACs can be reformulated as a time-derivative matrix element

$$\sigma_{ji} = \langle \varphi_j | \frac{\partial}{\partial t} | \varphi_i \rangle \,. \tag{4}$$

To run the dynamics, one needs to know NACs at every point along the trajectory. Since they are usually difficult to calculate in quantum chemistry, time-derivative matrix elements are often approximated by the overlap of the wavefunctions at two adjacent points along the trajectory:[S5]

$$\sigma_{ji}\left(t + \frac{\Delta}{2}\right) \approx \frac{\langle \varphi_j(t) | \varphi_i(t+\Delta) \rangle - \langle \varphi_j(t+\Delta) | \varphi_i(t) \rangle}{2\Delta}, \tag{5}$$

where $\Delta$ is the time step along the trajectory. In the adiabatic representation, the hopping probability in the FSSH method is computed as

$$P_{ij} = \max\left(0, \frac{2\Delta\,\mathrm{Re}(\rho_{ij})\sigma_{ij}}{\rho_{ii}}\right), \tag{6}$$

where $\rho_{ij} \equiv c_i c_j^*$ is the density matrix element.

We used the JADE package for conducting the FSSH non-adiabatic molecular dynamics[S6] along with the Firefly quantum chemistry package[S7] for obtaining electronic energies, energy gradients and wavefunctions overlap.

In order to compute the overlap between the wavefunctions we implemented a straightforward procedure[S8] using the Löwdin's formula. If the CASSCF wavefunctions are expanded in terms of Slater determinants $D_{ij\ldots}^{ab\ldots}$

$$\phi_\chi(t) = \sum_{ijab\ldots} C_{ij\ldots}^{ab\ldots} D_{ij\ldots}^{ab\ldots}, \quad \phi_\eta(t+\Delta) = \sum_{i'j'a'b'\ldots} C_{i'j'\ldots}^{a'b'\ldots} D_{i'j'\ldots}^{a'b'\ldots}, \tag{7}$$

the calculation of their overlap is reduced to the calculation of the overlap between the Slater determinants:

$$\left\langle D_{ij\ldots}^{ab\ldots} \middle| D_{i'j'\ldots}^{a'b'\ldots} \right\rangle = \det \begin{bmatrix} \langle\alpha|\alpha\rangle & 0 \\ 0 & \langle\beta|\beta\rangle \end{bmatrix}, \tag{8}$$

where $|\alpha\rangle$ and $|\beta\rangle$ denote the orbitals occupied by $\alpha$- and $\beta$-electrons, respectively.

In the case of the LZBL approach, the probability of non-adiabatic transitions is calculated in the following way:

$$P_{ij} = \exp\left(-\frac{\pi}{2\hbar}\sqrt{\frac{Z_{ij}^3}{\ddot{Z}_{ij}}}\right) \tag{9}$$

where $Z_{ij} = |U_j - U_k|$ is the adiabatic splitting of the potential energy surfaces.

Due to its simplicity and reliability, the LZBL method was implemented in various packages[S9–S11] for nonadiabatic dynamics simulations. The LZBL dynamics simulations presented in this paper were conducted within the MLatom package.[S9]

# 7 Dataset construction and neural network potentials

Training data for the neural network potentials consisted of 480 nonadiabatic molecular dynamics trajectories, initiated in the $S_2$ state and calculated at the SA(3)-CASSCF(12,12)/aug-cc-pVDZ level of theory. Targeted sampling around the newly discovered $\sigma\pi*/S_0$ conical intersection was achieved by supplementing this dataset with configurations generated via geodesic interpolation[S2] between configurations from the trajectories and the $\sigma\pi*/S_0$ minimum-energy conical intersection. From the trajectories, we identified 30,000 configurations with relatively small interatomic distances and randomly selected a subset of 1,000. For each of these, a geodesic scan was constructed using 15 intermediate points, generating a total of 15,000 new configurations. These were subsequently added to the original dataset.

The sets of 480 trajectories and 1,000 geodesic scans were split into training, validation, and test subsets with a ratio of 90:5:5. The subsets for training $S_0$, $S_1$, and $S_2$ models contained 69,440; 52,332; and 20,631 configurations, respectively. The dataset was split at the trajectory level, ensuring that entire trajectories were assigned to either the training, validation, or test subsets. This strict separation is crucial because the geometric variance between trajectories ($\sim$0.1 Å) is an order of magnitude larger than the variance within a single trajectory ($\sim$0.01 Å). Consequently, the test set contains genuinely unseen nuclear configurations, guaranteeing a valid assessment of the model's predictive power.

The Multi Atomic Cluster Expansion (MACE) architecture[S12] as implemented in the PyTorch library[S13] was employed to approximate potential energy surfaces of the methaniminium cation; each electronic state was considered independently. The models were trained with the following hyperparameters: a maximum spherical harmonics order of 3, 128 embedding channels, and a radial cutoff of 5.0 Å. Training was performed for 1125 epochs using stochastic weight averaging.[S14] The loss function coefficients for energy and forces were set to 1:100 for the first 1125 epochs, then changed to 1000:100 for a subsequent 375 epochs. The learning rates for these two stages were $10^{-2}$ and $10^{-3}$, respectively. The batch size was set to 32. The detailed information on predictive performance is provided in Figure S10.

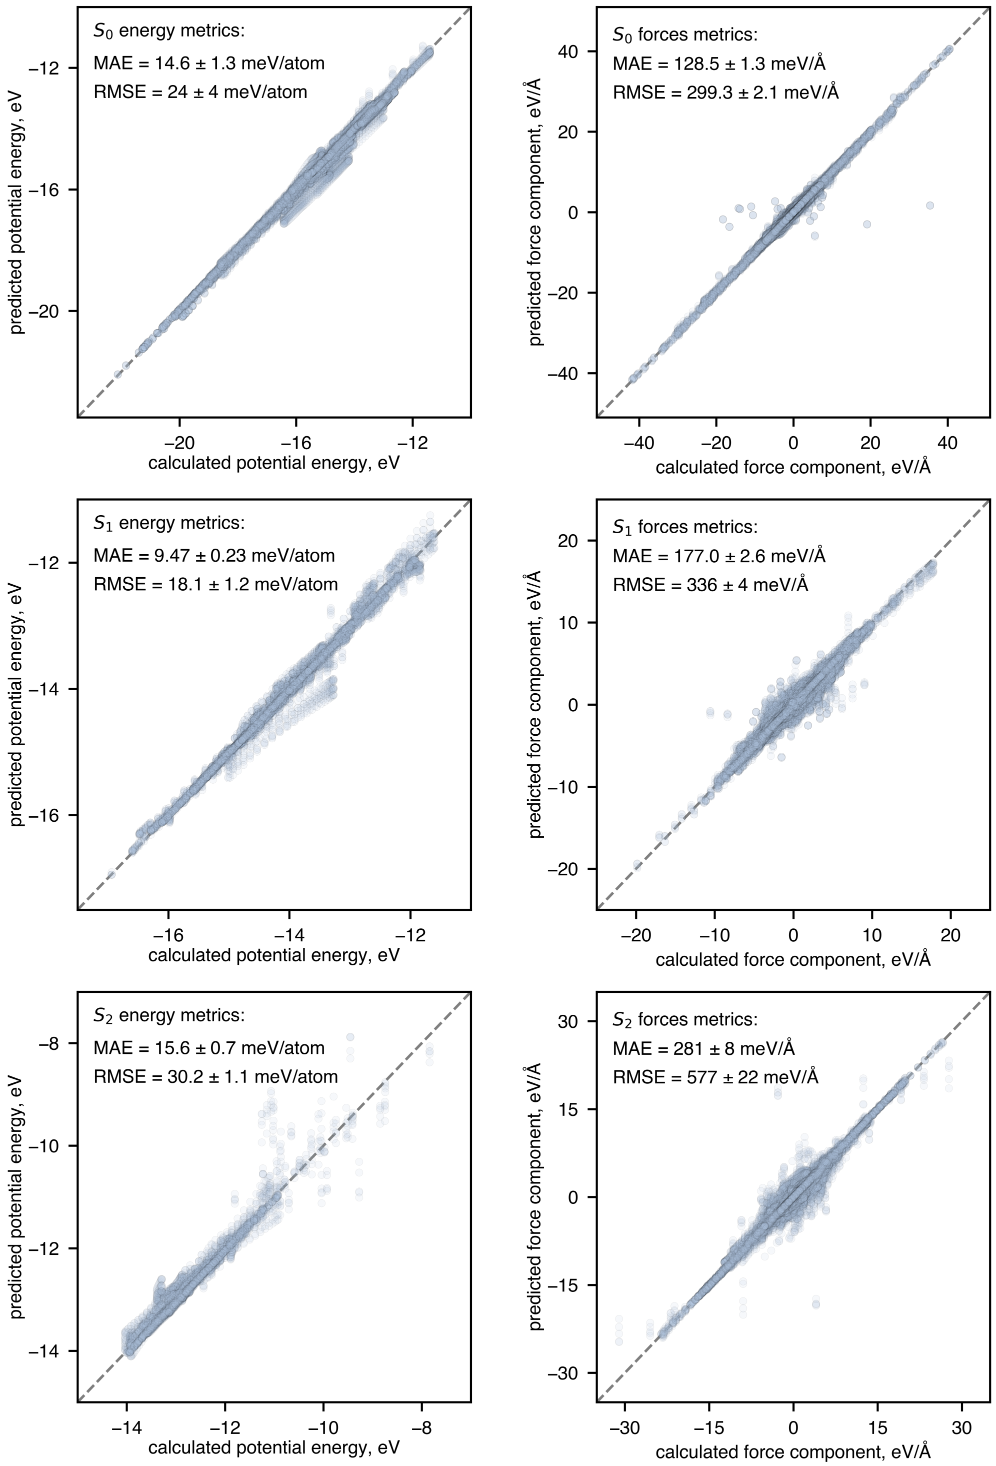


Figure S10: Predictive performance of the neural network interatomic potentials. Reported are the mean absolute error (MAE) and root-mean-square error (RMSE), presented as mean ± standard deviation (MEAN ± SD) from five-model ensembles.

# 8 Analysis of photodissociation channels

The resulting trajectories were divided into seven groups:

1. $CH_2NH_2$ dissociation into $CH_2^+$ and $NH_2$ through cleavage of the CN bond
2. Concerted elimination of two hydrogen atoms from the carbon center, forming $CNH_2^+$
3. Concerted elimination of two hydrogen atoms from the nitrogen center, forming $NCH_2^+$
4. Elimination of the hydrogen atom from the carbon center, forming $HCNH_2^+$
5. Elimination of the hydrogen atom from the nitrogen center, forming $H_2CNH^+$
6. Consecutive elimination of two hydrogen atoms from C and N, forming $HCNH^+$
7. $CH_2NH_2^+$ does not dissociate on the simulation timescale

We assigned trajectories starting in the $S_2$ state to different groups according to the following procedure:

1. For each trajectory, the CN bond distance ($d_{\mathrm{CN}}$) was computed at every time step. If the maximum value exceeded 3.7 Å ($\max d_{\mathrm{CN}} > 3.7$ Å), the trajectory was placed in the first group.
2. For each remaining trajectory, the maximum value of $f_{\mathrm{CH_2}}$ was calculated:

$$f_{\mathrm{CH_2}} = \left[\frac{1}{2} \cdot \left(\frac{d_{\mathrm{CH^1}}}{d_{\mathrm{CH^2}}} + \frac{d_{\mathrm{CH^2}}}{d_{\mathrm{CH^1}}}\right)\right]^{-1} \cdot d_{\mathrm{H}^{12}_{cm}\mathrm{C}},$$

   where $d_{\mathrm{CH}^i}$ is the distance from the C atom to one of the H atoms which are bonded to the C atom at the equilibrium geometry; $d_{\mathrm{H}^{12}_{cm}}$ is the distance from the center of mass of these hydrogen atoms to the C atom. The trajectories, for which $\max f_{\mathrm{CH_2}} >$ 1.75 Å, were placed in the second group.

3. For each remaining trajectory, the maximum value of $f_{\mathrm{NH}_2}$ was calculated:

$$f_{\mathrm{NH}_2} = \left[\frac{1}{2} \cdot \left(\frac{d_{\mathrm{NH}^3}}{d_{\mathrm{NH}^4}} + \frac{d_{\mathrm{NH}^4}}{d_{\mathrm{NH}^3}}\right)\right]^{-1} \cdot d_{\mathrm{H}^{34}_{cm}\mathrm{N}}$$

   where $d_{\mathrm{NH}^i}$ is the distance from the N atom to one of the hydrogen atoms which are bonded to the N atom at the equilibrium geometry; $d_{\mathrm{H}^{34}_{cm}}$ is the distance from the center of mass of these hydrogen atoms to the N atom. The trajectories, for which $\max f_{\mathrm{NH}_2} > 1.5$ Å, were placed in group 3.

4. For remaining trajectories, the values of the two distances $d_{\mathrm{CH}^1}$ and $d_{\mathrm{CH}^2}$ were computed at every time step. If the maximum value of one of these distances exceeded 1.8 Å, the trajectory was placed in group 4, except for those trajectories that also satisfied the conditions for being placed in group 5.

5. Similarly, if for any of the trajectories remaining after steps 1-3 the maximum value of one of the two distances $d_{\mathrm{NH}^3}$ and $d_{\mathrm{NH}^4}$ exceeded 1.8 Å, the trajectory was placed in group 5, except for those trajectories that also satisfied the conditions for being placed in group 4.

6. If the trajectory simultaneously satisfied the conditions of groups 4 and 5, it was assigned to group 6.

7. All remaining trajectories were assigned to group 7.

We assigned trajectories starting in the $S_1$ state to different groups by applying the same procedure with varied numerical criteria:

1. For each trajectory, if $\max d_{\mathrm{CN}} > 2.32$ Å, the trajectory was placed in group 1.

2. For each remaining trajectory, if $\max f_{\mathrm{CH}_2} > 2.0$ Å, it was placed in group 2.

3. For each remaining trajectory, if $\max f_{\mathrm{NH}_2} > 1.52$ Å, it was placed in group 3.

4. Those trajectories, for which the maximum value of either $d_{\mathrm{CH}^1}$ or $d_{\mathrm{CH}^2}$ was larger than 1.8 Å and which were not assigned to group 5, were placed in group 4.

5. Those trajectories, for which the maximum value of either $d_{\mathrm{NH}^1}$ or $d_{\mathrm{NH}^2}$ was larger than 1.9 Å and which were not assigned to group 3, were placed in group 5.

6. If the trajectory simultaneously satisfied the conditions of groups 4 and 5, it was assigned to group 6.

7. All remaining trajectories were assigned to group 7.

The cutoff values were established based on the temporal variation of the described parameters throughout the trajectories. The results for the dynamics starting in $S_2$ and $S_1$ are shown in Figures S11 and S12, respectively.

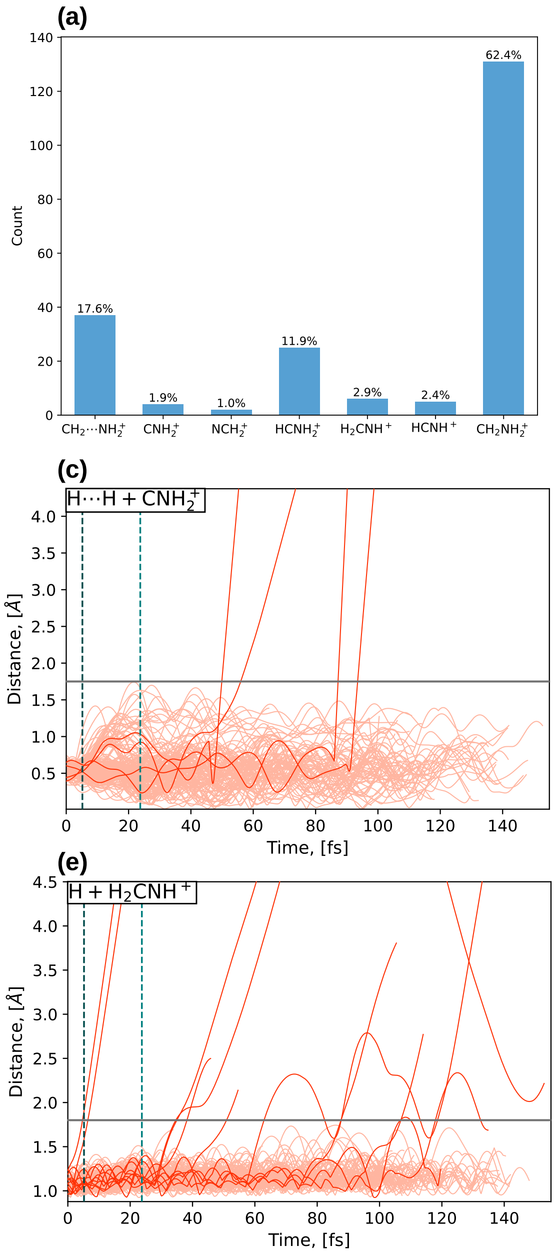


Figure S11: Analysis of photoproducts for the dynamics initiated in the $S_2$ state: (a) Fraction of trajectories following each dissociation pathway (see the main text for details); (b)-(f) Time dependence of the characteristic distance parameters for each group along each individual trajectory: $d_{\mathrm{CN}}$ (b), $f_{\mathrm{CH_2}}$ (c), $f_{\mathrm{NH_2}}$ (d), the largest of $d_{\mathrm{NH^1}}$ and $d_{\mathrm{NH^2}}$ (e), the largest of $d_{\mathrm{CH^1}}$ and $d_{\mathrm{CH^2}}$ (f). The vertical dashed lines represent the average transition times to $S_1$ (darker lines) and $S_0$ (lighter lines). The horizontal lines show the cutoff values for the corresponding parameters.

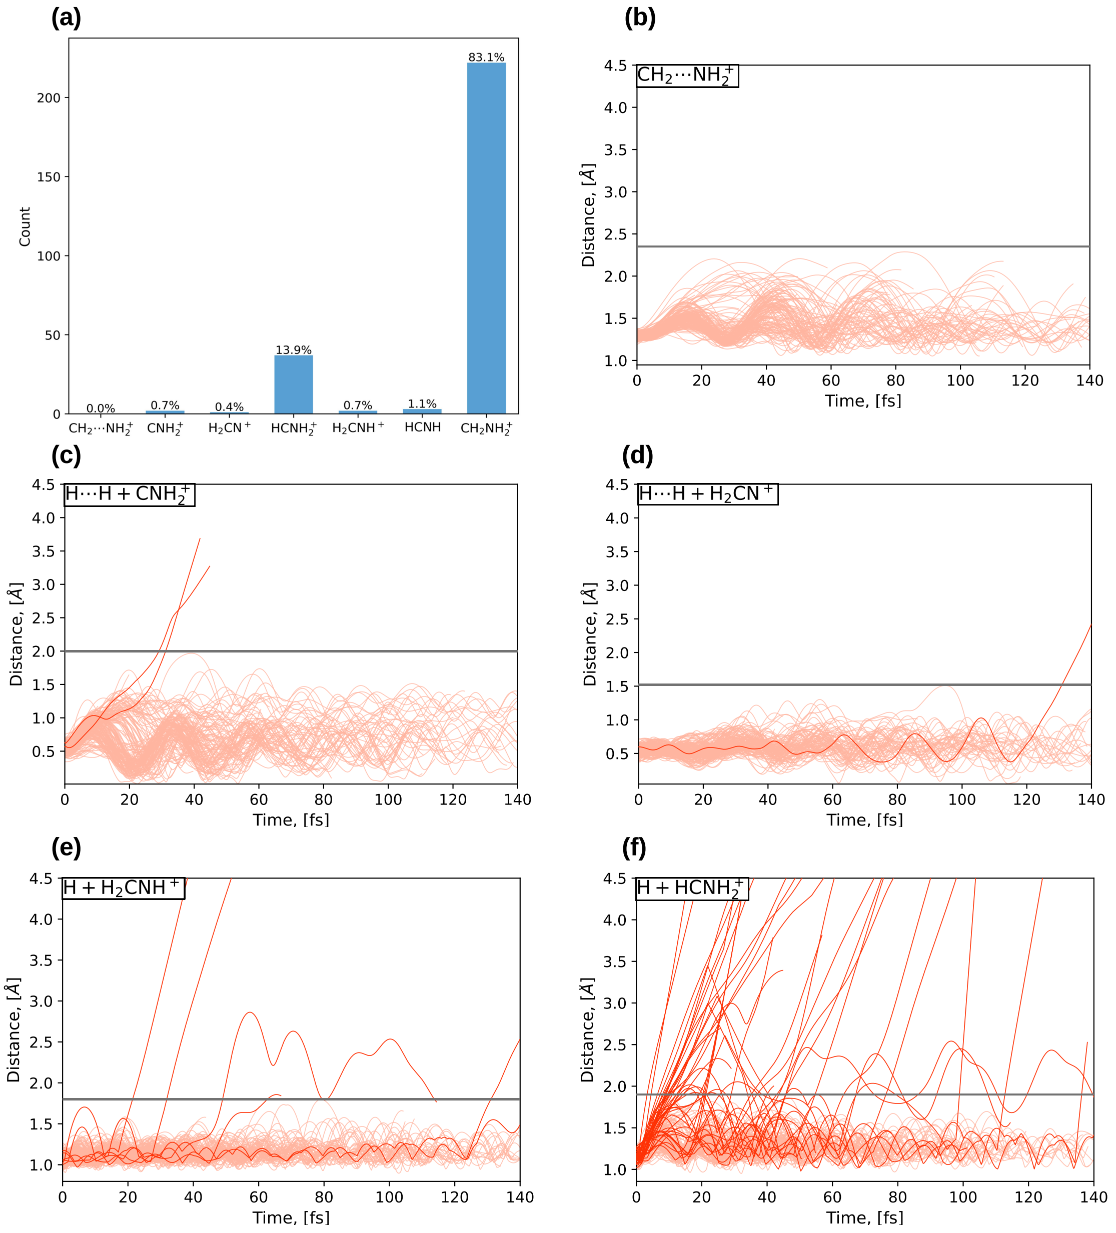


Figure S12: Analysis of photoproducts for the dynamics initiated in the $S_1$ state: (a) Fraction of trajectories following each dissociation pathway (see the main text for details); (b)-(f) Time dependence of the characteristic distance parameters for each group along each individual trajectory: $d_{\mathrm{CN}}$ (b), $f_{\mathrm{CH_2}}$ (c), $f_{\mathrm{NH_2}}$ (d), the largest of $d_{\mathrm{NH^1}}$ and $d_{\mathrm{NH^2}}$ (e), the largest of $d_{\mathrm{CH^1}}$ and $d_{\mathrm{CH^2}}$ (f). The horizontal lines show the cutoff values for the corresponding parameters.

# 9 Temporal evolution of photodissociation channels

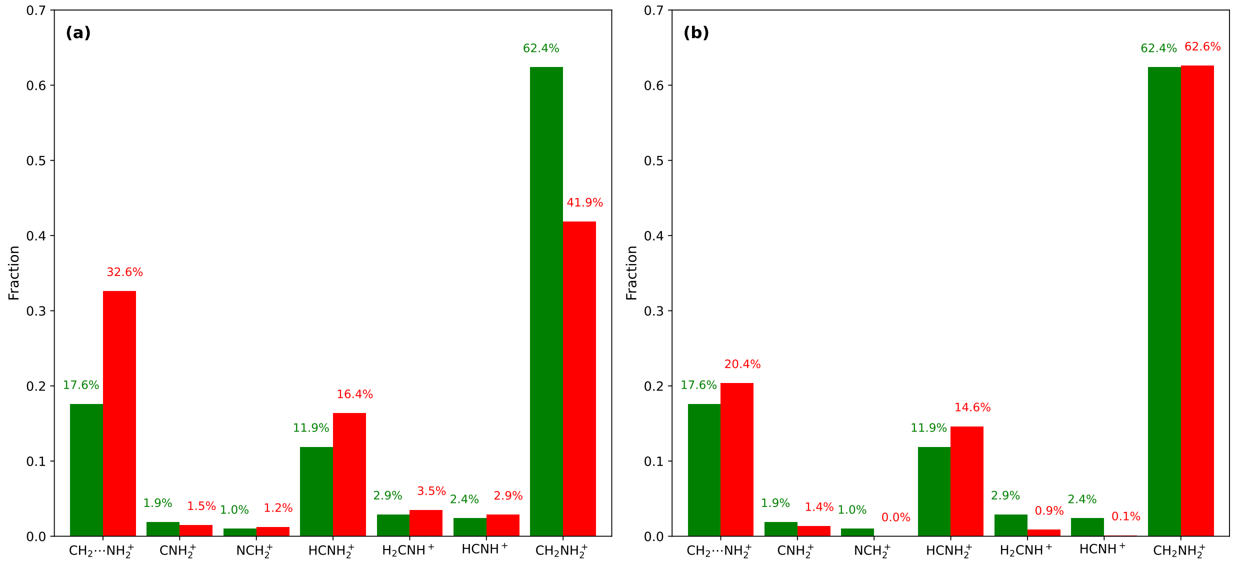


Figure S13: Branching ratios for photodissociation pathways initiated in the $S_2$ state. Results are shown for ML/LZBL dynamics (red, 800 trajectories) with trajectory cutoffs of 100 fs (a) and 50 fs (b) and compared to on-the-fly CASSCF/FSSH dynamics with an average trajectory length of 56 fs (green, 400 trajectories).

# 10 ML analysis of excited-state decay through MECIs

## 10.1 Locating MECIs with the ML potential

The neural network potential, which we constructed based on the dataset from the CASSCF/FSSH molecular dynamics, is used to identify the conical intersection through which the system decays from $S_1$ to $S_0$. We conduct the minimization of the following Lagrangian:

$$\mathcal{L} = E_{S_0} + E_{S_1} + \lambda(E_{S_0} - E_{S_1}), \tag{10}$$

where $E_{S_0}$ and $E_{S_1}$ are the adiabatic energies of the $S_0$ and $S_1$ states, respectively. The minimization starts from the molecular geometry, where the hop from $S_1$ to $S_0$ occurs during dynamics simulation. The optimization is performed using the SLSQP method from the SciPy package.[S15] The idea is that if the hop takes place near the particular conical intersection, the optimization should converge toward the geometry of this conical intersection. As a result, the hop can be assigned to that particular conical intersection.

## 10.2 Geometries of MECIs from the ML potential

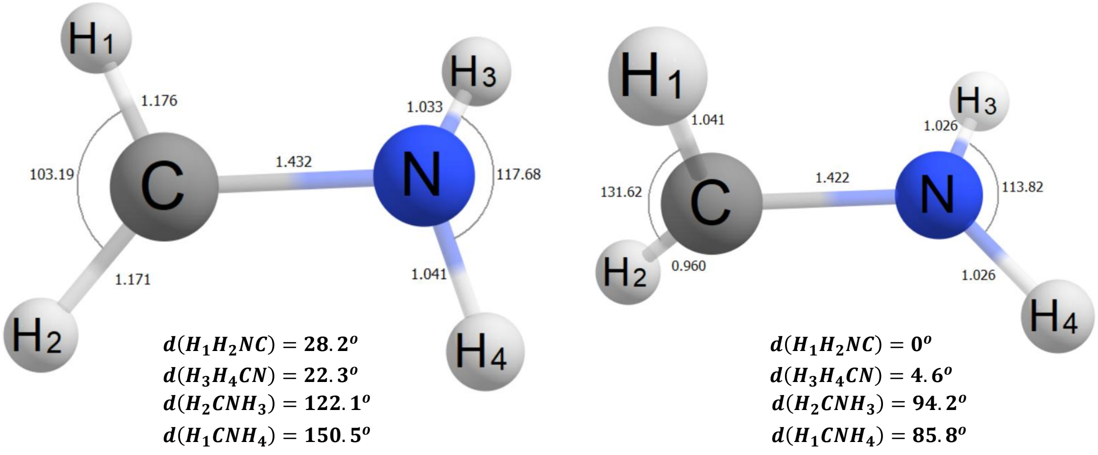


Figure S14: Geometries of the $S_2/S_1$ (left) and $\pi\pi^*/S_0$ (right) MECIs, located using the neural network potential. The root-mean-square deviation between the MECIs located by CASSCF and the ML potential is 0.1 Å.

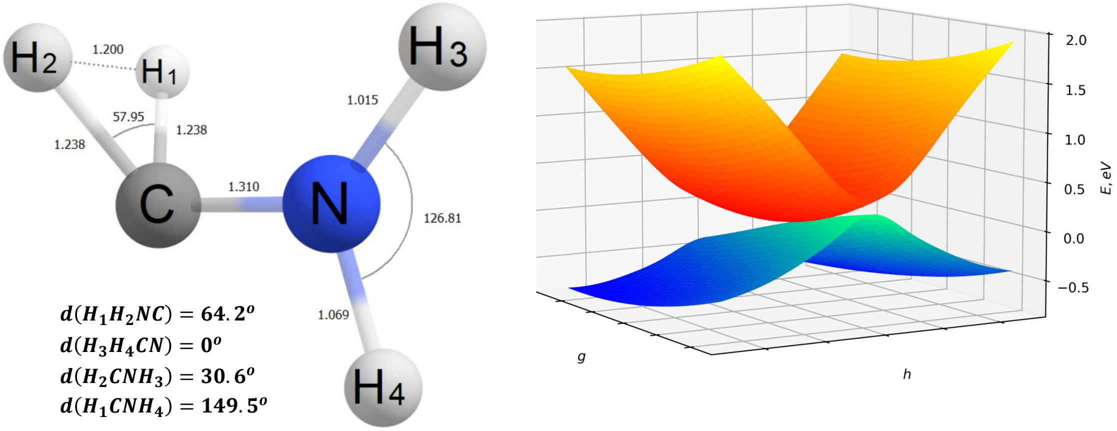


Figure S15: Left: Geometry of the $\sigma\pi^*/S_0$ MECI located using the neural network potential. Right: Potential energy surfaces in the branching plane around the MECI. The root-mean-square deviation between the MECIs located by CASSCF and the ML potential is 0.08 Å.

## 10.3 Energies of MECIs from the ML potential

Table S2: Comparison of MECI relative energies calculated at the CASSCF/aug-cc-pVDZ level and with the CASSCF-based neural network potentials. Energies are given in eV with respect to the ground-state equilibrium geometry. Based on an ensemble of five models, the machine learning uncertainty is 0.01 eV in the vicinity of all three conical intersections. The difference between the *ab initio* and ML energies falls within 0.1 eV, consistent with the predictive performance of the neural network interatomic potentials (see Fig. S10).

| | $S_2/S_1$ | $\sigma\pi^*/S_0$ | $\pi\pi^*/S_0$ |
|---|---|---|---|
| ML | 8.17 | 6.29 | 3.62 |
| CASSCF | 8.15 | 6.24 | 3.73 |

## 10.4 Statistical uncertainty of the ML-based branching ratios

The branching ratios reported in Table 1 of the main text for the CASSCF/FSSH simulations from the $S_1$ state were obtained by averaging over 300 trajectories. Of these, 186 were sufficiently long to transition to the $S_0$ state, and for each, the conical intersection nearest to the hop configuration was located. To estimate the statistical uncertainty of calculated branching ratios, we used 5,000 trajectories, simulated using neural network potentials. From this large set, ten random samples of 186 trajectories were selected, and the standard deviation of their branching ratios was computed. These results, including uncertainty estimates, are reported in Table 1 of the main text.

# 11 Ab initio and ML population dynamics

Figure S16 shows the population dynamics after $S_1$ and $S_2$ photoexcitation, obtained using CASSCF and neural network potentials. The ML/LZBL and CASSCF/FSSH dynamics show good agreement at early times, but diverge progressively at longer simulation times. The divergence arises from two factors: the inherent dispersion of trajectories over time (shaded areas), which occurs even with the same potential, and the additional divergence caused by differences between the ML and *ab initio* potentials.

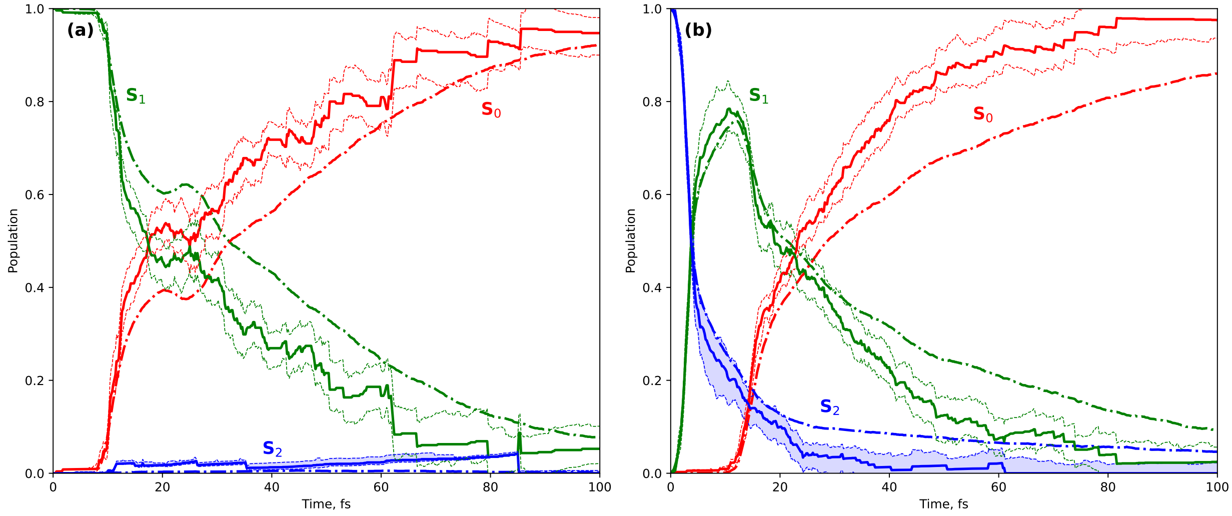


Figure S16: Time evolution of electronic states populations for the dynamics initiated in the $S_1$ (a) and $S_2$ (b) states. The solid lines show the average from on-the-fly CASSCF/FSSH dynamics simulations, using 300 trajectories for $S_1$ and 400 for $S_2$. The dash-dotted lines represent the average over 5,000 trajectories from LZBL dynamics simulations using the MACE-fitted neural network potentials. The shaded regions around the solid lines indicate the dispersion of the population estimates over 300 ($S_1$) and 400 ($S_2$) trajectories. These dispersions are calculated based on the simulations with the neural network potentials.

To further assess the robustness of the neural network potentials in sampling configurational space, out-of-sample diagnostics were performed during the ML/LZBL simulations. The application of correction protocols to the ML-based dynamics provides a clear improvement over the raw, uncorrected results. The details are presented in Section 12.

## 12 Assessing robustness in ML dynamics

To further assess the robustness of the neural network potentials in sampling configurational space, out-of-sample diagnostics were performed during the massive ML/LZBL simulations. An ensemble of five neural network models was trained for each electronic state using identical datasets and hyperparameters, differing only in their random weight initialization (see Section 7). We used the standard deviation of the ensemble's energy predictions to quantify the potential energy fit uncertainty for each geometry. Using a threshold of 100 meV – consistent with the overall fit quality (Fig. S10) – we analyzed the trajectories preceding a hop to $S_0$. For the 5,000 trajectories initiated in $S_2$, the ensemble's standard deviation remained below this threshold for 93% of geometries in $S_2$ and 94.6% in $S_1$. Similarly, for trajectories initiated in $S_1$, 97.3% of geometries exhibited a standard deviation below the threshold.

To further enhance the reliability of population predictions in non-adiabatic dynamics using neural network potentials, we explicitly incorporate the model's uncertainty in our weighting algorithm. We have implemented two slightly different protocols to identify and handle trajectories entering under-sampled or sparsely populated regions of the configuration space. In the first protocol (**P-1**), a trajectory is discarded from the average if the uncertainty of the ML models, as quantified by the ensemble standard deviation, exceeds a certain threshold value at any time step prior to a hop to $S_0$.

The second protocol (**P-2**) is formulated as follows. For each trajectory, we construct a discrete indicator function for each electronic state. The value of the function is 1 if the system is in that particular state at a given time step, and 0 otherwise. The average population of a state is then the mean value of its corresponding indicator function over the ensemble of trajectories:

$$p_{S_j}(t) = \frac{\sum_{i=1}^{N} w_i(t) \cdot \mathbf{1}_{S_j}(t)}{\sum_{j=1}^{K} \sum_{i=1}^{N} w_i(t) \cdot \mathbf{1}_{S_j}(t)}, \tag{11}$$

where $p_{S_j}(t)$ is the average population of state $S_j$ at time $t$, $\mathbf{1}_{S_j}$ is the indicator function

for state $S_j$, $w_i$ is the weight of trajectory $i$, $N$ is the total number of trajectories, and $K$ is the number of electronic states. To prioritize trajectories with more reliable energy predictions, we assign each a weight inversely proportional to the standard deviation of the neural network ensemble. When all trajectory weights are set to unity, Eq. 11 reduces to the standard average, where the population of a given electronic state is simply the fraction of trajectories propagating on that state.

The application of both correction protocols (**P-1** and **P-2**) to the ML-based dynamics shows consistent time-dependence and provides a clear improvement over the raw, uncorrected results, as evidenced in Figs. S17 and S18 for the dynamics initiated in the $S_1$ and $S_2$ states, respectively.

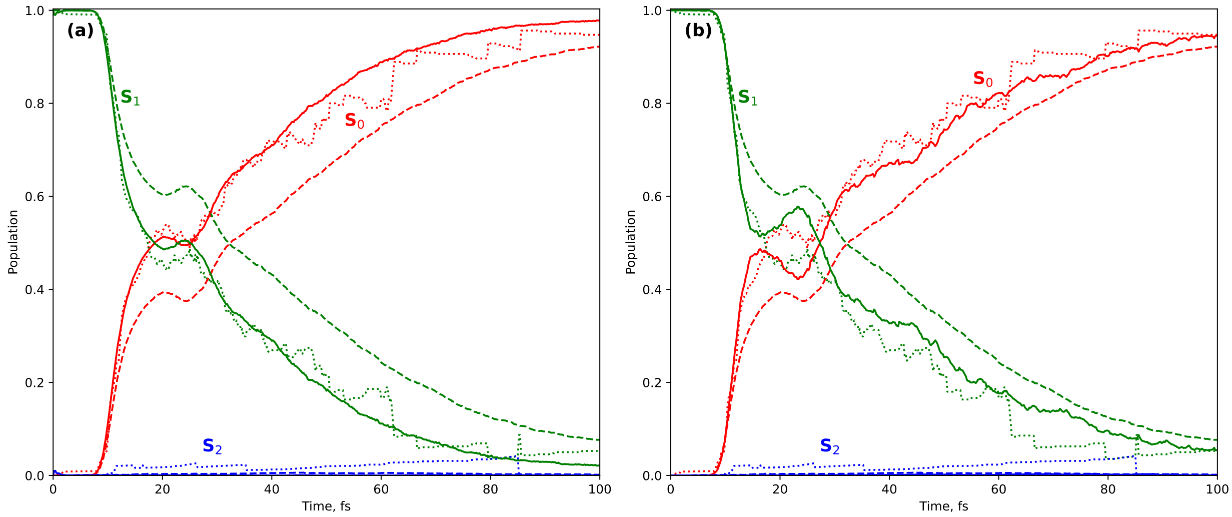


Figure S17: Time evolution of electronic states populations for the dynamics initiated in the $S_1$ state. The dotted lines show the average over 300 trajectories from on-the-fly CASSCF/FSSH dynamics simulations. The dashed lines represent the average over 5,000 trajectories from LZBL dynamics simulations using the MACE-fitted neural network potentials. Solid lines represent the average from the simulations with neural network potentials, corrected for the ML model uncertainty using protocols **P-1** (a) and **P-2** (b). A cutoff value of 85 meV was used for procedure **P-1**.

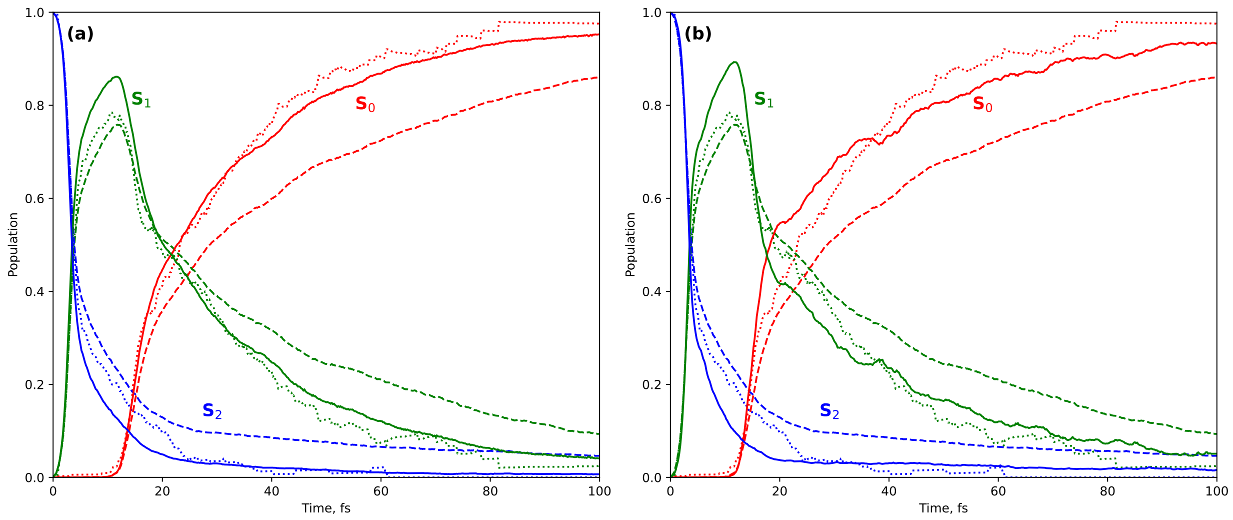


Figure S18: Time evolution of electronic states populations for the dynamics initiated in the $S_2$ state. The dotted lines show the average over 400 trajectories from on-the-fly CASSCF/FSSH dynamics simulations. The dashed lines represent the average over 5,000 trajectories from LZBL dynamics simulations using the MACE-fitted neural network potentials. Solid lines represent the average from the simulations with neural network potentials, corrected for the ML model uncertainty using protocols **P-1** (a) and **P-2** (b). A cutoff value of 110 meV was used for procedure **P-1**.

# 13 Branching ratios of final products from $S_1$ decay

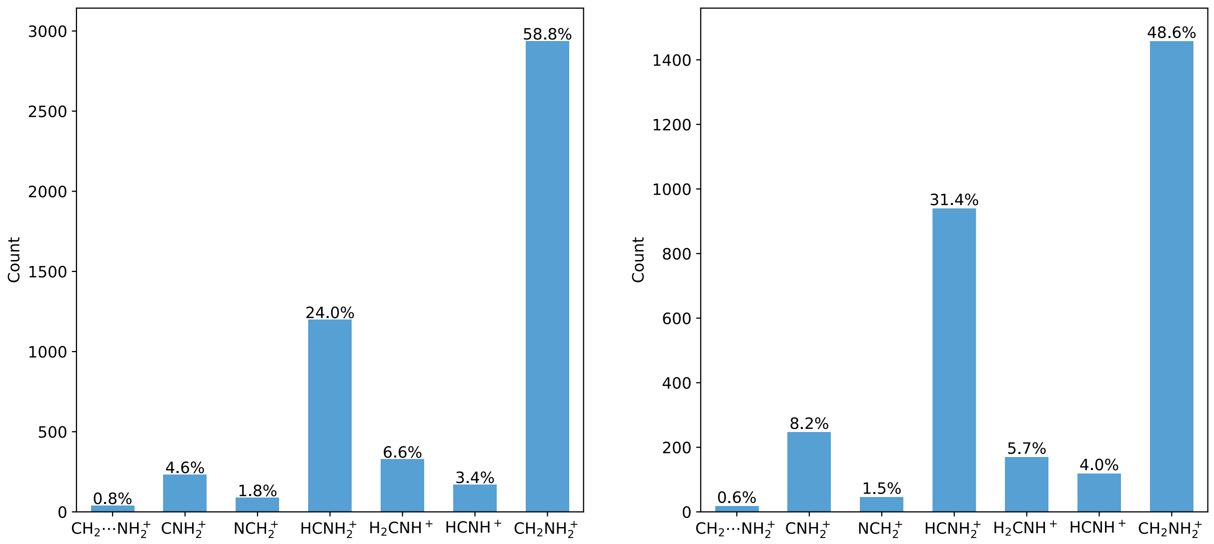


Figure S19: Branching ratios of final products from $S_1$ decay: no vibrational pre-excitation (left) and with pre-excitation of the $CH_2$ wagging mode (right). Branching ratios are determined from ML/LZBL dynamics by analyzing products formed within 100 fs along 5,000 (no pre-excitation) and 3,000 (with pre-excitation) trajectories. The threshold values are 3.12 Å (CN bond cleavage); 1.52 Å (double H-atom subtraction from the carbon center); 1.78 Å (double H-atom subtraction from the nitrogen center); 2.01 Å (single H-atom subtraction from the carbon center); 1.7 Å (single H-atom subtraction from the nitrogen center). For details, see Section S8.

# 14 Infrared absorption spectrum

Table S3: Vibrational frequencies and infrared absorption intensities of $CH_2NH_2^+$ at the $S_0$ minimum computed at the MP2/aug-cc-pVDZ level of theory. The values in brackets are the SA(3)-CASSCF(12,12)/aug-cc-pVDZ frequencies used to sample initial conditions for the dynamics simulations. Note that the out-of-plane twisting mode is IR-inactive.

| No. | Mode | Symmetry | Frequency $cm^{-1}$ | Intensity $Debye^2/(amu \cdot Å^2)$ |
|---|---|---|---|---|
| 1 | in-plane twisting | $B_2$ | 938 (938) | 4.2251 |
| 2 | out-of-plane $NH_2$ wagging | $B_1$ | 959 (963) | 0.1187 |
| 3 | out-of-plane twisting | $A_2$ | 1086 (1083) | 0.0000 |
| 4 | out-of-plane $CH_2$ wagging | $B_1$ | 1167 (1089) | 0.8591 |
| 5 | in-plane rocking | $B_2$ | 1348 (1338) | 0.1794 |
| 6 | in-plane $CH_2$ scissoring | $A_1$ | 1462 (1418) | 0.3778 |
| 7 | in-plane CN stretching | $A_1$ | 1597 (1565) | 0.7656 |
| 8 | in-plane $NH_2$ scissoring | $A_1$ | 1764 (1741) | 1.1551 |
| 9 | in-plane $CH_2$ sym. stretching | $A_1$ | 3200 (3062) | 0.3317 |
| 10 | in-plane $CH_2$ asym. stretching | $B_2$ | 3339 (3189) | 0.5173 |
| 11 | in-plane $NH_2$ sym. stretching | $A_1$ | 3483 (3398) | 3.9312 |
| 12 | in-plane $CH_2$ asym. stretching | $B_2$ | 3611 (3512) | 4.5108 |

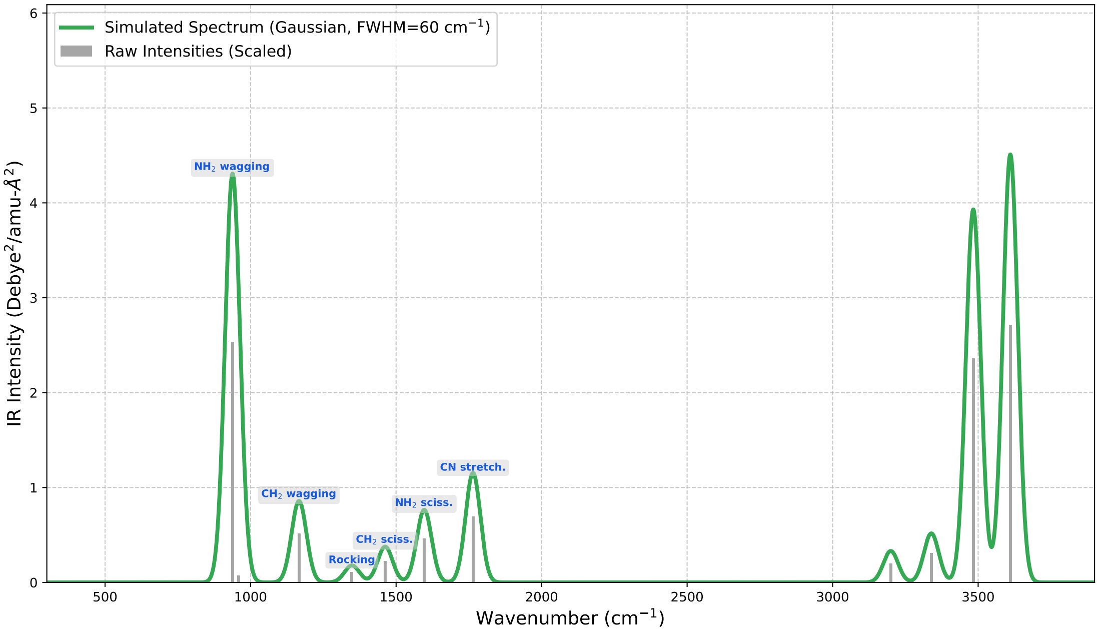


Figure S20: Simulated IR spectrum of $CH_2NH_2^+$. Note that the $CH_2$ wagging mode is IR-active and can be pumped independently of the other modes.

# References

(S1) Barbatti, M.; Aquino, A. J.; Lischka, H. Ultrafast two-step process in the non-adiabatic relaxation of the $CH_2NH_2$ molecule. *Mol. Phys.* **2006**, *104*, 1053–1060.

(S2) Zhu, X.; Thompson, K. C.; Martínez, T. J. Geodesic interpolation for reaction pathways. *J. Chem. Phys.* **2019**, *150*.

(S3) Tully, J. C. Molecular dynamics with electronic transitions. *J. Chem. Phys.* **1990**, *93*, 1061–1071.

(S4) Belyaev, A. K.; Lebedev, O. V. Nonadiabatic nuclear dynamics of atomic collisions based on branching classical trajectories. *Phys. Rev. A* **2011**, *84*, 014701.

(S5) Hammes-Schiffer, S.; Tully, J. C. Proton transfer in solution: Molecular dynamics with quantum transitions. *J. Chem. Phys.* **1994**, *101*, 4657–4667.

(S6) Du, L.; Lan, Z. An On-the-Fly Surface-Hopping Program JADE for nonadiabatic molecular dynamics of polyatomic systems: implementation and applications. *J. Chem. Theory Comput.* **2015**, *11*, 1360–1374, PMID: 26574348.

(S7) Granovsky, A. A. Firefly version 8. `http://classic.chem.msu.su`, Accessed on October 14, 2025.

(S8) Pittner, J.; Lischka, H.; Barbatti, M. Optimization of mixed quantum-classical dynamics: Time-derivative coupling terms and selected couplings. *Chem. Phys.* **2009**, *356*, 147–152.

(S9) Zhang, L.; Pios, S. V.; Martyka, M.; Ge, F.; Hou, Y.-F.; Chen, Y.; Chen, L.; Jankowska, J.; Barbatti, M.; Dral, P. O. MLAtom software ecosystem for surface hopping dynamics in Python with quantum mechanical and machine learning methods. *J. Chem. Theory Comput.* **2024**, *20*, 5043–5057.

(S10) Menger, M. F.; Ehrmaier, J.; Faraji, S. PySurf: A framework for database accelerated direct dynamics. *J. Chem. Theory Comput.* **2020**, *16*, 7681–7689.

(S11) Shakiba, M.; Smith, B.; Li, W.; Dutra, M.; Jain, A.; Sun, X.; Garashchuk, S.; Akimov, A. Libra: A modular software library for quantum nonadiabatic dynamics. *Softw. Impacts* **2022**, *14*, 100445.

(S12) Batatia, I.; Kovacs, D. P.; Simm, G.; Ortner, C.; Csányi, G. MACE: Higher order equivariant message passing neural networks for fast and accurate force fields. *Adv. Neural Inf. Process Syst.* **2022**, *35*, 11423–11436.

(S13) Paszke, A.; Gross, S.; Massa, F.; Lerer, A.; Bradbury, J.; Chanan, G.; Killeen, T.; Lin, Z.; Gimelshein, N.; Antiga, L.; others Pytorch: An imperative style, high-performance deep learning library. *Adv. Neural Inf. Process Syst.* **2019**, *32*.

(S14) Izmailov, P.; Podoprikhin, D.; Garipov, T.; Vetrov, D.; Wilson, A. G. Averaging weights leads to wider optima and better generalization. 34th Conference on Uncertainty in Artificial Intelligence 2018, UAI 2018. 2018; pp 876–885.

(S15) Virtanen, P.; Gommers, R.; Oliphant, T. E.; Haberland, M.; Reddy, T.; Cournapeau, D.; Burovski, E.; Peterson, P.; Weckesser, W.; Bright, J.; van der Walt, S. J.; Brett, M.; Wilson, J.; Millman, K. J.; Mayorov, N.; Nelson, A. R. J.; Jones, E.; Kern, R.; Larson, E.; Carey, C. J.; Polat, İ.; Feng, Y.; Moore, E. W.; VanderPlas, J.; Laxalde, D.; Perktold, J.; Cimrman, R.; Henriksen, I.; Quintero, E. A.; Harris, C. R.; Archibald, A. M.; Ribeiro, A. H.; Pedregosa, F.; van Mulbregt, P.; SciPy 1.0 Contributors SciPy 1.0: Fundamental Algorithms for Scientific Computing in Python. *Nat. Methods* **2020**, *17*, 261–272.
